# Supplementary material for: Dexterous Non-Prehensile Manipulation for Ungraspable Object via Extrinsic Dexterity
Source: arXiv:2503.23120 source file (2025-03-29)
Supplement: Supplementary file 1 [file domain_randomization.tex]

\begin{table}[thbp]
\caption{Domain randomization of Wall and Edge task.}
\centering
            \begin{tabular}{c|c|c|c}
            \toprule
            % \rowcolor[HTML]{D4F7EE}
            Parameter & Type & Distribution & Initial Range\\
            \midrule
            
            \rowcolor[HTML]{EFEFEF} 

            \multicolumn{4}{l}{\textbf{Robot}} \\
            Mass & Scaling & $ \textrm{uniform}$ & [0.5, 1.5] \\ %
            Friction & Scaling & $ \textrm{uniform}$ & [0.7, 1.3] \\
           Joint Lower Limit & Scaling & $ \textrm{loguniform}$ & [0.0, 0.01] \\ %
            Joint Upper Limit & Scaling & $ \textrm{loguniform}$ & [0.0, 0.01] \\
            Joint Stiffness & Scaling & $ \textrm{loguniform}$ & [0.0, 0.01] \\
            Joint Damping & Scaling & $ \textrm{loguniform}$ & [0.0, 0.01] \\

            \rowcolor[HTML]{EFEFEF} 
            \multicolumn{4}{l}{\textbf{Object}} \\
            Mass & Scaling & $ \textrm{uniform}$ & [0.5, 1.5]  \\
            Friction & Scaling & $ \textrm{uniform}$ & [0.5, 1.5] \\
            Scale & Scaling & $ \textrm{uniform}$ & [0.95, 1.05] \\
            Position Noise & Additive & $ \textrm{gaussian}$ & [0.0, 0.02] \\
            Rotation Noise & Additive & $ \textrm{gaussian}$ & [0.0, 0.2] \\
            
            \rowcolor[HTML]{EFEFEF} 
            \multicolumn{4}{l}{\textbf{Observation}} \\
            Obs Correlated. Noise & Additive & $ \textrm{gaussian}$ & [0.0, 0.001] \\
            Obs Uncorrelated. Noise & Additive & $ \textrm{gaussian}$ & [0.0, 0.002] \\

            \rowcolor[HTML]{EFEFEF} 
            \multicolumn{4}{l}{\textbf{Action}} \\
            Action Correlated Noise & Additive & $ \textrm{gaussian}$ & [0.0, 0.015]  \\
            Action Uncorrelated Noise & Additive & $ \textrm{gaussian}$ & [0.0, 0.05] \\

            \rowcolor[HTML]{EFEFEF} 
            \multicolumn{4}{l}{\textbf{Environment}} \\
            Gravity & Additive & $ \textrm{normal}$ & [0, 0.4] \\

            \bottomrule
            \end{tabular}
    
     \label{tab:dr}
\end{table}
