# Supplementary material for: Dexterous Non-Prehensile Manipulation for Ungraspable Object via Extrinsic Dexterity
Source: arXiv:2503.23120 source file (2025-03-29)
Supplement: Supplementary file 3 [file obs_push.tex]

\begin{table}[thbp]
    \centering
    
    \caption{Observation space of RL Policy in simulation.}
    \begin{tabular}{c|c}
    \toprule
    % \rowcolor[HTML]{D4F7EE}
    Index & Description\\\hline
    0 - 17 & arm-hand dof position\\\hline
    18 - 32 & hand fingertip position\\\hline
    33 - 36 & hand base position\\\hline
    37 - 43 &	object position, rotation\\\hline
    44 - 49 & object linear velocity, angle velocity\\\hline
    50 - 52 & contact target position\\\hline
    53 - 55 & push target position \\\hline
    
    % \bottomrule
    \end{tabular}
    
    \label{tab:obs_push}
\end{table}
