# Supplementary material for: Dexterous Non-Prehensile Manipulation for Ungraspable Object via Extrinsic Dexterity
Source: arXiv:2503.23120 source file (2025-03-29)
Supplement: Supplementary file 4 [file obs_wall.tex]

\begin{table*}[!t]
    \centering
    \caption{Observation space of Push Policy.}
    \begin{tabular}{c|c}
    \toprule
    % \rowcolor[HTML]{D4F7EE}
    Index & Description\\\hline
    0 - 60 & right arm-hand dof position, velocity\\\hline
    60 - 120 & left arm-hand dof position, velocity\\\hline
    120 - 133 & right hand end-effector position, velocity, linear velocity, angle velocity\\\hline
    133 - 146 &	left hand end-effector position, velocity, linear velocity, angle velocity\\\hline
    146 - 159 &	object base position, rotation, linear velocity, angle velocity\\\hline
    159 - 172 &	articulated object top part position, rotation, linear velocity, angle velocity\\\hline
    172 - 185 &	articulated object bottom part position, rotation, linear velocity, angle velocity\\\hline
    185 - 187 &	object dof position, velocity\\\hline
    % 187 - 257 & desired object motion trajectory $G = (\bm{g}_t,\bm{g}_{t+1},..., \bm{g}_{t+T})$\\\hline
    % 257 - 397 & sequence of 6-DoF wrist actions $(\bm{a}^W_t,\bm{a}^W_{t+1},..., \bm{a}^W_{t+T})$ generated by high-level planner\\\hline
    397 - 462 & right hand fingertip pose, linear velocity, angle velocity\\\hline
    462 - 527 & left hand fingertip pose, linear velocity, angle velocity\\
    \bottomrule
    \end{tabular}
    
    \label{tab:obs_wall}
\end{table*}
